# Supplementary material for: Chiral superfluid states in hybrid graphene heterostructures
Source: arXiv:1207.1440 source file (2013-08-29)
Supplement: Supplementary file 1 [file supplemental_material.pdf]

# Supplemental Material to "Chiral superfluid states in hybrid graphene heterostructures"

Below we first briefly address the issue of how intervalley scattering might modify our results and then present the results for the dynamical density-density response function.

At low energies the two valleys are decoupled and therefore within the low-energy theory one obtains two independent exciton condensates for the two valleys with two midgap states, one for each valley. In the presence of an axial gauge fiels a vortex will be present in both valleys. The effect of intervalley interactions is to slightly split the two midgap modes [1]. The fact that the two valleys have chiral condensates with opposite chirality does not affect the presence of midgap states.

To discuss how the dynamical density-density response function is sensitive to the chirality of the exciton condensate, without loss of generality, we can consider the following simplified Hamiltonian

$$H_{\mathbf{k}} = \begin{pmatrix} \varepsilon_{\mathbf{k},1} & -\Delta^{\perp}_{\mathbf{k}} \\ -\left(\Delta^{\perp}_{\mathbf{k}}\right)^* & \varepsilon_{\mathbf{k},2} \end{pmatrix} \tag{1}$$

where $\Delta^{\perp}_{\mathbf{k}} = \Delta_0 e^{-\frac{(k-k_F)^2}{2\sigma^2}} e^{iJ\theta_{\mathbf{k}}}$ is modeled by a Gaussian around the original Fermi vector in the non-interaction system, and $J = 0$ for the non-chiral condensate and $J = 1, -1$ for the chiral condensates at the two valleys. The dynamical density-density response function (at $T = 0$) is given by [2, 3]

$$\chi(\mathbf{q}, \omega) = \sum_{\lambda,\lambda'} \int \frac{d^2\mathbf{k}}{(2\pi)^2} \frac{n_{\lambda,\mathbf{k}} - n_{\lambda',\mathbf{k}+\mathbf{q}}}{\omega + E_{\lambda}(\mathbf{k}) - E_{\lambda'}(\mathbf{k}+\mathbf{q}) + i\eta} \left| \Psi^{\dagger}_{\lambda}(\mathbf{k}) \hat{P} \Psi_{\lambda'}(\mathbf{k}+\mathbf{q}) \right|^2 \tag{2}$$

where $\lambda, \lambda' = \pm$ refer to the eigenenergy bands of (1) with eigenenergies $E_{\pm}(\mathbf{k})$ and eigenvectors $\Psi_{\pm}(\mathbf{k})$, $n_{\lambda,\mathbf{k}}$ is the Fermi function, and the operator $\hat{P} = 1$ stands for the symmetric (density-sum) response and $\hat{P} = \sigma_z$ for the antisymmetric (density-difference) response. Given that the two layers are quite close to each other, the symmetric response is the most physical one [2, 3]. We show the numerical results for the symmetric response function below. Clearly, the results for the $J = 1$ and the $J = -1$ chiral states are the same, i.e., the two chiral condensates at the two valleys have the same dynamical response, as expected. The response $\chi(\mathbf{q})$ at $\omega = 0.1\Delta_0$ (left panel), $\omega = 2\Delta_0$ (middle panel), and $\omega = 2.7\Delta_0$ (right panel) are shown in Fig. 1, where $\Delta_0 = 0.075\gamma_1$ and $\sigma = 0.1k_0$ adopted from Fig. 3 in the main text. The responses in the chiral and non-chiral states are mostly distinct around $\omega = 2\Delta_0$ with a much stronger response appearing in the chiral states as shown in the middle panel of the figure.

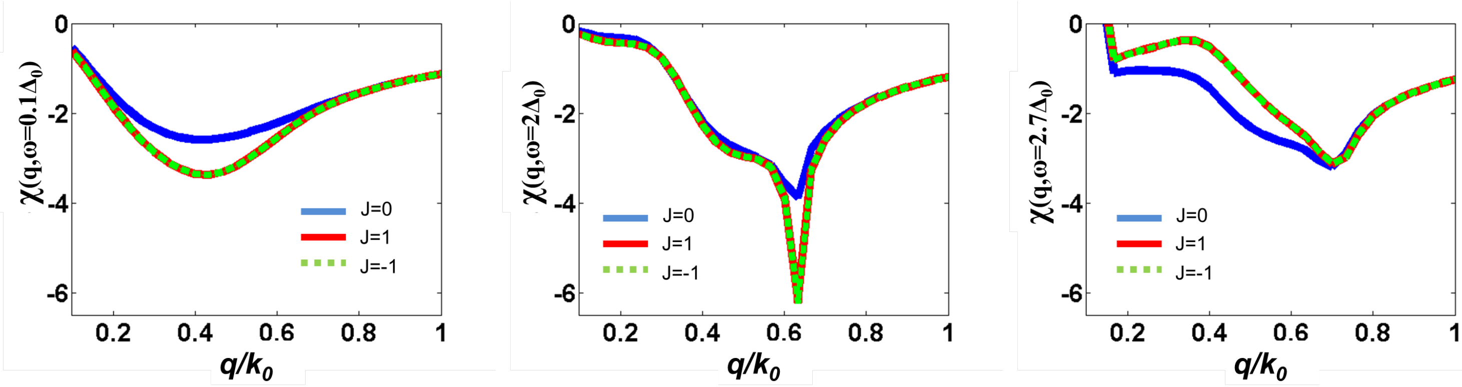


Figure 1: Response function $\chi(\mathbf{q})$ at $\omega = 0.1\Delta_0,\ 2\Delta_0,\ 2.7\Delta_0$ in the non-chiral $J = 0$ (blue solid line) and chiral $J = 1$ (red solid line) $J = -1$ (green dashed line) states, with $\Delta_0 = 0.075\gamma_1$ and $\sigma = 0.1k_0$ adopted from Fig. 3 in the main text ($k_0 \equiv \gamma_1/(\hbar v_F)$ is the momentum scale defined in the main text). A sharp feature appears in the chiral states at $\omega = 2\Delta_0$ as shown in the middle papel.

## References

[1] B. Seradjeh, H. Weber, and M. Franz, Phys. Rev. Letts **101**, 246404 (2008).

[2] G. Borghi, M. Polini, R. Asgari, and A. H. MacDonald, Phys. Rev. B **82**, 155403 (2010).

[3] C. Triola and E. Rossi, Phys. Rev. B **86**, 161408(R) (2012).
